# Supplementary material for: Supercell Wannier functions and a faithful low-energy model for Bernal bilayer graphene
Source: arXiv:2407.02576 source file (2024-11-09)
Supplement: Supplementary file 1 [file supp.pdf]

# Supplementary Material:
# Supercell Wannier functions and a faithful low-energy model for Bernal bilayer graphene

Ammon Fischer,[1,*] Lennart Klebl,[2,*] Dante M. Kennes,[1,3] and Tim O. Wehling[2,4]

[1]Institute for Theory of Statistical Physics, RWTH Aachen University, and JARA Fundamentals of Future Information Technology, 52062 Aachen, Germany
[2]I. Institute for Theoretical Physics, Universität Hamburg, NotkestraSSe 9-11, 22607 Hamburg, Germany
[3]Max Planck Institute for the Structure and Dynamics of Matter, Center for Free Electron Laser Science, 22761 Hamburg, Germany
[4]The Hamburg Centre for Ultrafast Imaging, 22761 Hamburg, Germany

(Dated: November 9, 2024)

## CONTENTS

I. Construction of the supercell Hamiltonian from first principles 1
II. Supercell Wannierization via single-shot projection 2
III. Supercell Wannier functions for Bernal bilayer graphene 3
IV. Supercell Wannier functions for monolayer graphene 4
V. Supercell wannier functions for rhombohedral (ABC) trilayer graphene 5
VI. Dual-gated Ohno-Coulomb interaction 5
VII. Valley as quantum number 7
References 8

## I. CONSTRUCTION OF THE SUPERCELL HAMILTONIAN FROM FIRST PRINCIPLES

The microscopic Hamiltonian for Bernal bilayer graphene (BBG) is taken from Ref. [44] and is obtained from first principles via density functional theory (DFT) and successive Wannierization of the carbon $p_z$-orbitals located at the sublattices $X \in \{A_1, B_1, A_2, B_2\}$ within the primitive cell. The carbon $p_z$-orbitals are located at $\boldsymbol{\tau}_{A_1} = {}^1\!/\!_3\boldsymbol{a}_1 + {}^1\!/\!_3\boldsymbol{a}_2$, $\boldsymbol{\tau}_{B_1} = {}^2\!/\!_3\boldsymbol{a}_1 + {}^2\!/\!_3\boldsymbol{a}_2$, $\boldsymbol{\tau}_{A_2} = {}^1\!/\!_3\boldsymbol{a}_1 + {}^1\!/\!_3\boldsymbol{a}_2 + \tau_2 + d\boldsymbol{e}_z$ and $\boldsymbol{\tau}_{B_2} = {}^2\!/\!_3\boldsymbol{a}_1 + {}^2\!/\!_3\boldsymbol{a}_2 + \tau_2 + d\boldsymbol{e}_z$ within the primitive cell. Here, $\boldsymbol{a}_1 = (\sqrt{3}/2, 1/2)^{\mathrm{T}}$ and $\boldsymbol{a}_2 = (0, 1)^{\mathrm{T}}$ labels Bravais lattice vectors of the real-space primitive cell, $d$ denotes the interlayer distance of bilayer graphene [44] and $\tau_2 = {}^1\!/\!_3\boldsymbol{a}_1 + {}^1\!/\!_3\boldsymbol{a}_2$ is the lateral shift of the first layer with respect to the second layer. We further model the presence of an external displacement field $\Delta$ that lifts the inversion symmetry via the following term in the Hamiltonian:

$$\mathsf{H}_\Delta = \frac{\Delta}{2} \sum_{\boldsymbol{r}} \left( c^\dagger_{\boldsymbol{r},A_1} c_{\boldsymbol{r},A_1} + c^\dagger_{\boldsymbol{r},B_1} c_{\boldsymbol{r},B_1} - c^\dagger_{\boldsymbol{r},A_2} c_{\boldsymbol{r},A_2} - c^\dagger_{\boldsymbol{r},B_2} c_{\boldsymbol{r},B_2} \right), \tag{1}$$

where $\boldsymbol{r} = n_1\boldsymbol{a}_1 + n_2\boldsymbol{a}_2$ labels translations of the primitive unit cell. The microscopic Hamiltonian is extended to the superlattice with re-scaled lattice vectors $\boldsymbol{A}_i = n_i\boldsymbol{a}_i$ by exploiting translational invariance on the two length scales, i.e., the carbon-carbon scale $\boldsymbol{\delta} = n_1\boldsymbol{a}_1 + n_2\boldsymbol{a}_2$, $n_i \in \{0, \dots, n_s - 1\}$ and the supercell scale $\boldsymbol{\Delta} = \tilde{n}_1\boldsymbol{A}_1 + \tilde{n}_2\boldsymbol{A}_2$, $\tilde{n}_i \in \mathbb{Z}$. To this end, we may write the microscopic Hamiltonian as

$$H_{XX'}(\boldsymbol{k}) = \sum_{\boldsymbol{\Delta}\boldsymbol{\delta}} e^{-i\boldsymbol{k}(\boldsymbol{\Delta}+\boldsymbol{\delta})} t_{XX'}(\boldsymbol{\Delta} + \boldsymbol{\delta}), \qquad \mathsf{H} = \sum_{\boldsymbol{k},X,X'} c^\dagger_{\boldsymbol{k},X} H_{XX'}(\boldsymbol{k}) c_{\boldsymbol{k},X'}, \tag{2}$$

* These authors contributed equally.

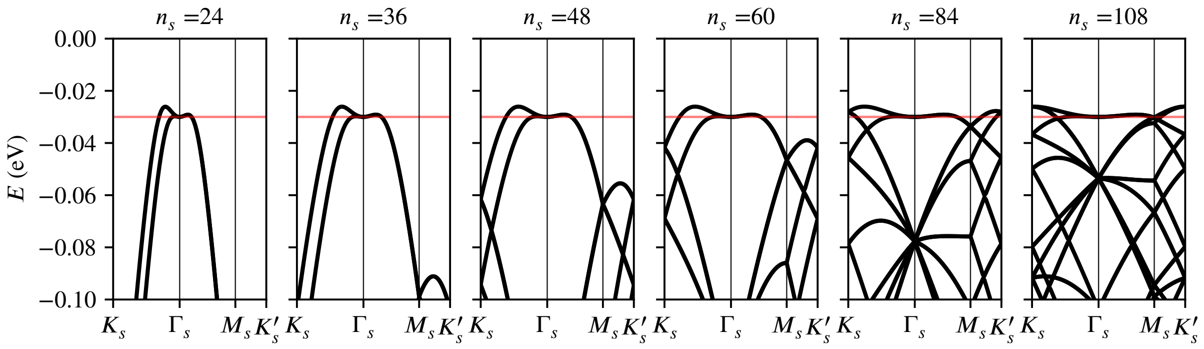


FIG. 1. Supercell bandstructure obtained for different scaling factors $n_s$ in the presence of an interlayer potential difference of $\Delta = 60$ meV. The red horizontal line indicates the position of the VHS.

where $\boldsymbol{k}$ refers to crystal momenta in the first Brillouin zone (BZ) of the microscopic lattice, and $t_{XX'}(\boldsymbol{\delta})$ are the hopping elements of the original (microscopic) Wannier Hamiltonian given in Ref. [44]. An inverse Fourier transform on the microscopic scale associated with $(\boldsymbol{\delta}, \boldsymbol{k})$ yields the elements of the supercell Hamiltonian at mini-BZ momentum $\boldsymbol{K}$:

$$\begin{aligned} H_{X,X'+\tilde{\delta}}(\boldsymbol{K}) &= \sum_{\boldsymbol{G}} e^{i\boldsymbol{G}\tilde{\boldsymbol{\delta}}} H_{XX'}(\boldsymbol{K}+\boldsymbol{G}) \\ &= \sum_{\boldsymbol{G}} \sum_{\boldsymbol{\Delta\delta}} e^{i\boldsymbol{G}\tilde{\boldsymbol{\delta}}} e^{-i(\boldsymbol{K}+\boldsymbol{G})(\boldsymbol{\Delta}+\boldsymbol{\delta})} t_{XX'}(\boldsymbol{\Delta}+\boldsymbol{\delta}) \\ &= \sum_{\boldsymbol{\Delta\delta}} \delta_{\tilde{\boldsymbol{\delta}},\boldsymbol{\delta}} e^{-i\boldsymbol{K}(\boldsymbol{\Delta}+\boldsymbol{\delta})} t_{XX'}(\boldsymbol{\Delta}+\boldsymbol{\delta}) \\ &= e^{-i\boldsymbol{K}\tilde{\boldsymbol{\delta}}} \sum_{\boldsymbol{\Delta}} e^{-i\boldsymbol{K}\boldsymbol{\Delta}} t_{XX'}(\boldsymbol{\Delta}+\tilde{\boldsymbol{\delta}})\,. \end{aligned} \tag{3}$$

Here, reciprocal lattice vectors of the primitive cell/supercell are denoted by $\boldsymbol{g} = b_1\boldsymbol{g}_1 + b_2\boldsymbol{g}_2$ and $\boldsymbol{G} = \tilde{b}_1\boldsymbol{G}_1 + \tilde{b}_2\boldsymbol{G}_2$, respectively. In practice, the supercell Hamiltonian can therefore be constructed by setting up the microscopic Hamiltonian $H_{XX'}(\boldsymbol{k})$ on an equidistant mesh with $n_s \times n_s$ momentum points that is shifted by the mini-BZ momentum $\boldsymbol{K}$. An inverse Fourier transform (in conjunction with a proper unraveling of the $4n_s^2$ indices associated with the microscopic carbon $p_z$-orbitals that reside within the supercell) then yields the supercell Hamiltonian defined in Eq. (3). We note that the supercell Hamiltonian obtained by virtue of Fourier transformations differs in its gauge compared to the Wannier Hamiltonian defined in Eq. (2). This is because the Fourier transformation in Eq. (2) does not involve the (microscopic) positions of the carbon atoms within the primitive cell $\boldsymbol{r}_X$ such that eigenstates of the Hamiltonian obey momentum space periodicity via $\psi_{\boldsymbol{k}+\boldsymbol{g},b}(\boldsymbol{r}) = \psi_{\boldsymbol{k},b}(\boldsymbol{r})$. The phase factor $\exp(-i\boldsymbol{K}\tilde{\boldsymbol{\delta}})$ in the definition of the supercell Hamiltonian violates aforementioned momentum space periodicity, which however can be restored explicitly by a unitary gauge transformation.

The bandstructure for supercells with different choices of the scaling factor $n_s$ is shown in Fig. 1 along the irreducible path of the concomitant mini-BZ. The red line indicates the position of the van-Hove singularity. The Wannierization scheme proposed in the main text remains valid as long as two single bands (one per valley) contribute to the Fermi surface, which marks a breakdown criterion at $n_s \sim 60$, i.e. where the supercell lattice constant $L_s \sim 1/|\boldsymbol{q}_s|$ becomes comparable to the extend of the Fermi surface pockets at low electronic densities. For larger scaling factors additional bands appear in the vicinity of the Fermi energy requiring further supercell Wannier functions to capture their spectral weight.

## II. SUPERCELL WANNIERIZATION VIA SINGLE-SHOT PROJECTION

While implementations of the maximally localized Wannier function algorithm are readily available (e.g., Wannier90 [96]), creating symmetry adapted, maximally localized Wannier orbitals is in general more intriguing [92, 93]. We found that it is sufficient and more reliable[1] to construct Wannier functions manually by virtue of single-shot projections [68, 78, 94]. To this end, we consider a set of $\boldsymbol{J_k}$ Bloch bands, which we would like to find a Wannier representation for. If all target bands are isolated,

[1] We apply the particular Wannierization procedure outlined in this section to models with large unit cells (supercells), i.e., thousands of orbitals in a tight-binding formalism. It therefore requires optimized code to tackle the computational demand.

exactly $J_{\boldsymbol{k}} = N_\alpha$ Wannier orbitals are required to represent all bands in the target band manifold. However, Wannier functions can also be sampled from a larger set of Bloch bands $J_{\boldsymbol{k}} > N_\alpha$ within a given energy window, c.f. Fig. 1 (c) of the main text. In this case, the number of target Bloch states may additionally vary for each crystal momentum $\boldsymbol{k}$. We then start from $N_\alpha$ trial wavefunctions $g_{\boldsymbol{k}\alpha}(\boldsymbol{r})$, which we project onto the target band manifold:

$$|\phi_{\boldsymbol{k}\alpha}\rangle = \sum_{b\in J_{\boldsymbol{k}}} w^{\alpha}_{\boldsymbol{k}b} \, |\psi_{\boldsymbol{k}b}\rangle\langle\psi_{\boldsymbol{k}b} \, | \, g_{\boldsymbol{k}\alpha}\rangle = \sum_{b\in J_{\boldsymbol{k}}} A_{\alpha b}(\boldsymbol{k}) \, |\psi_{\boldsymbol{k}b}\rangle \ , \tag{4}$$

where $w^{\alpha}_{\boldsymbol{k}b} \in [0,1]$ are optional weighting factors, which can be tuned to achieve optimal disentanglement of the bands. The matrix of inner products $A_{\alpha b}(\boldsymbol{k})$ is rectangular with dimension $N_\alpha \times J_{\boldsymbol{k}}$. The projected wave functions $|\phi_{\boldsymbol{k}\alpha}\rangle$ are smooth in the momentum domain, but not orthonormal. Therefore, we next search for the best unitary approximation of $A_{\alpha b}(\boldsymbol{k})$ by performing an SVD $\hat{A} = \hat{U}\hat{\Sigma}\hat{V}^\dagger$ of the overlap matrix and defining

$$\hat{B} = \hat{A}\left[\hat{V}\left(\hat{\Sigma}^\dagger\hat{\Sigma}\right)^{-1/2}\hat{V}^\dagger\right] = \hat{A}\left[\hat{A}^\dagger\hat{A}\right]^{-1/2}, \tag{5}$$

where all matrices above are evaluated at the same crystal momentum $\boldsymbol{k}$. By replacing $A_{\alpha b}(\boldsymbol{k})$ with its unitary approximation $B_{\alpha b}(\boldsymbol{k})$ in Eq. (4), we obtain Löwdin-orthonormalized states

$$|\chi_{\boldsymbol{k}\alpha}\rangle = \sum_{\alpha=1}^{N_\alpha} B_{\alpha\beta}(\boldsymbol{k}) \, |\phi_{\boldsymbol{k}\beta}\rangle \ , \tag{6}$$

which are related to the original Bloch states $|\psi_{\boldsymbol{k}b}\rangle$ by a unitary transformation. The orthonormalized states $|\chi_{\boldsymbol{k}\alpha}\rangle$ retain a smooth gauge in $\boldsymbol{k}$ space and can therefore be cast to real-space Wannier functions by a (discrete) Fourier transformation.

For the graphitic models considered in the scope of this work, we find it convenient to do multiple iterations of the single-shot projection detailed above. Thereby we have the freedom of treating each *input* to an iteration as trial functions, allowing us to modify $|\chi_{\boldsymbol{k}\alpha}\rangle$ *before* the next iteration. We make use of this freedom by localizing the trial states with a Fermi cutoff, i.e.,

$$g(\boldsymbol{r},\alpha) = f\left(\frac{|\boldsymbol{r}| - d}{\sigma}\right)\chi(\boldsymbol{r},\alpha)\,, \tag{7}$$

where $d$ resembles the maximum spread of the new trial state, $\sigma$ the decay width, and $f(x) = (1+e^x)^{-1}$ is the Fermi function. As weighting functions $w^{\alpha}_{\boldsymbol{k}b}$, we choose asymmetric exponentials. The trial states corresponding to the conduction and valence bands, respectively, are weighted with

$$w^{\pm}_{\boldsymbol{k}b} = \begin{cases} \exp\left(-\dfrac{|\epsilon_{\boldsymbol{k}b} - E^{\pm}|}{\eta_{\text{intra}}}\right) & \text{iff} \quad \epsilon_{\boldsymbol{k}b} \in \epsilon^{\pm}\,, \\ \exp\left(-\dfrac{|\epsilon_{\boldsymbol{k}b} - E^{\mp}|}{\eta_{\text{inter}}}\right) & \text{iff} \quad \epsilon_{\boldsymbol{k}b} \in \epsilon^{\mp}\,. \end{cases} \tag{8}$$

Here, $\epsilon^{\pm}$ denotes the set of conduction (valence) bands, and $E^{\pm}$ is the conduction (valence) band edge. The widths of the exponentials, $\eta_{\text{intra}}$ and $\eta_{\text{inter}}$, determine whether the Haldane-like or a trivial Wannierization is found—we generally have to set $\eta_{\text{inter}} > \eta_{\text{intra}}$ to achieve sufficient inter-orbital coupling, which is responsible for the topology.

## III. SUPERCELL WANNIER FUNCTIONS FOR BERNAL BILAYER GRAPHENE

In order to generate exponentially localized Wannier functions, we perform the modified single-shot projection technique detailed in Section II, with a Fermi function cutoff at scale $d = 3L_s$ (with broadening $\sigma = L_s/2$). The number of steps performed is four in total, with the first three steps including the Fermi smoothening, and the last step being a genuine projection of a trial function. We choose the symmetric (asymmetric) exponential energy cutoffs as $\eta_{\text{intra}} = 0.1\,\text{eV}$ ($\eta_{\text{inter}} = 0.18\,\text{eV}$).Figure 2 (a) demonstrates that the resulting Wannier functions are exponentially localized. Most of the weight of the $\zeta = +$ ($\zeta = -$) Wannier orbital is concentrated on the non-dimer orbitals $B_2$ ($A_1$). In Fig. 2 (b), we further show the phase evolution of the supercell Wannier orbitals' envelope (i.e., canceling out the microscopic valley phase $e^{i\boldsymbol{K}^{v}\cdot\boldsymbol{r}}$), where a phase winding of $2\pi$ between the two sublattice components becomes apparent.

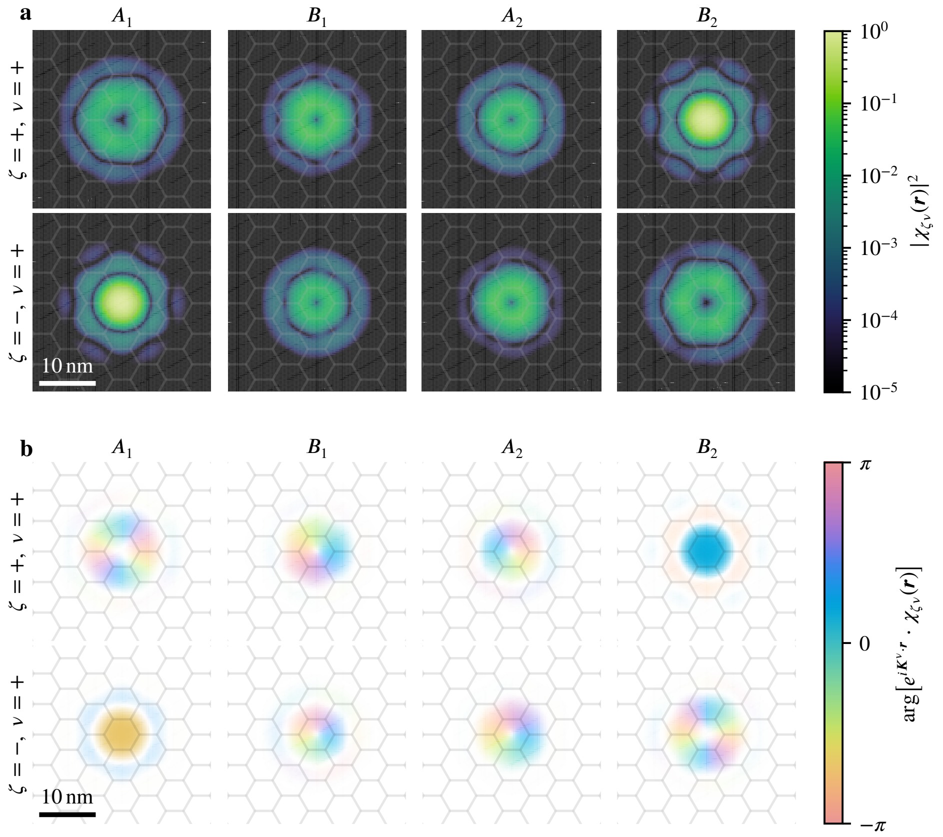


FIG. 2. Supercell Wannier functions of Bernal bilayer graphene under the influence of an electric displacement field $\Delta = 60\,\mathrm{meV}$. (a): Absolute value of the two Wannier functions in real space for valley $\nu = +$ on the four sublattices. (b) Complex phase evolution of the envelope function, i.e., without the microscopic phase stemming from the valley.

## IV. SUPERCELL WANNIER FUNCTIONS FOR MONOLAYER GRAPHENE

We model monolayer graphene with nearest- and next-nearest hopping parameters $t = -2.7\,\mathrm{eV}$, $t' = 0.1\,\mathrm{eV}$. We use a $n_s \times n_s = 24 \times 24$ supercell, with a momentum resultion of $N_{\boldsymbol{k}} = 18^2$ points in the mini-BZ. The inversion symmetry breaking gap is added to the Hamiltonian as

$$\mathsf{H}_\Delta = \Delta \sum_{\boldsymbol{r}} \left( c^\dagger_{\boldsymbol{r},A_1} c_{\boldsymbol{r},A_1} - c^\dagger_{\boldsymbol{r},B_1} c_{\boldsymbol{r},B_1} \right), \tag{9}$$

with $\Delta = 50\,\mathrm{meV}$. In order to generate exponentially localized Wannier functions, we perform the modified single-shot projection technique detailed in Section II, with a Fermi function cutoff at scale $d = 3L_s$ (with broadening $\sigma = L_s/3$). The number of steps performed is four in total, with the first three steps including the Fermi smoothening, and the last step being a genuine projection of a trial function. The spread of the gaussian test function is set to $0.3L_s$, and the symmetric (asymmetric) exponential energy cutoff is $\eta_{\mathrm{intra}} = 0.05\,\mathrm{eV}$ ($\eta_{\mathrm{inter}} = 0.15\,\mathrm{eV}$).

Figure 3 (a) demonstrates that the resulting Wannier functions are exponentially localized. Most of the weight of the $\zeta = +$ ($\zeta = -$) Wannier orbital is concentrated on the $A_1$ ($B_1$) sublattice. In Fig. 3 (b), we further show the phase evolution of the supercell Wannier orbitals' envelope (i.e., cancelling out the microscopic valley phase $e^{i\boldsymbol{K}^\nu\cdot\boldsymbol{r}}$), where a phase winding of $\pi$ between the two sublattice components becomes apparent. Panel (c) shows the resulting band structure of the projected model for valley $\nu = +$ (orange) compared to the microscopic bandstructure in the supercell (i.e., *both* valleys; gray).

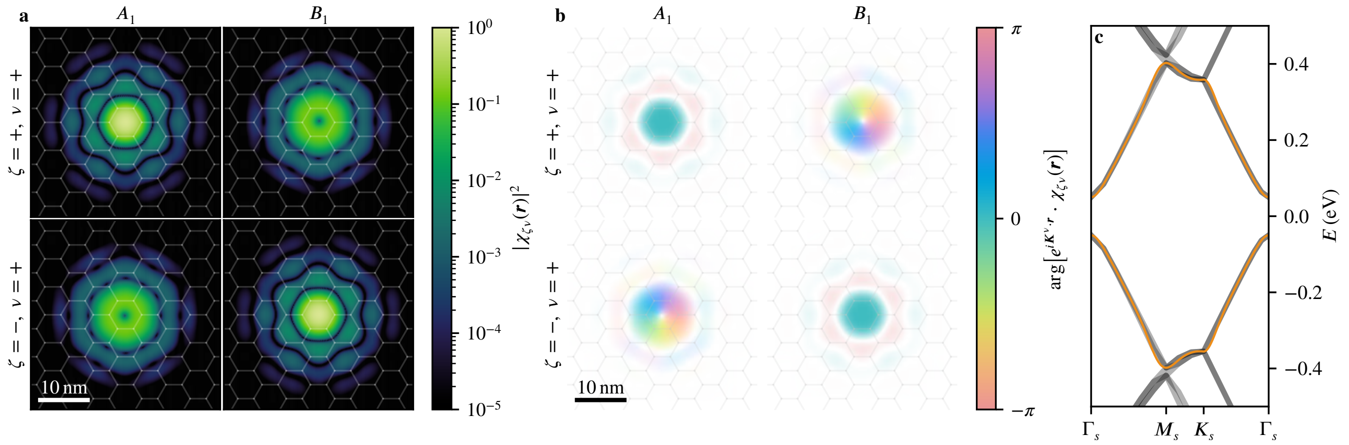


FIG. 3. Supercell Wannier functions of monolayer graphene under an inversion symmetry breaking field $\Delta = 50\,\text{meV}$. (a): Absolute value of the two Wannier functions in real space for valley $\nu = +$. (b): Complex phase evolution of the envelope function, i.e., without the microscopic phase stemming from the valley. (c): Band structure of the supercell model in *both* valleys (gray) and the wannierized model in valley $\nu = +$ (orange).

## V. SUPERCELL WANNIER FUNCTIONS FOR RHOMBOHEDRAL (ABC) TRILAYER GRAPHENE

The microscopic Hamiltonian for rhombohedral (ABC) trilayer graphene is taken from Ref. [97]. We add inversion symmetry breaking $\Delta$ via the following term in the Hamiltonian:

$$\mathsf{H}_\Delta = \frac{3\Delta}{2} \sum_{\boldsymbol{r}} \left( c^\dagger_{\boldsymbol{r},A_1} c_{\boldsymbol{r},A_1} + c^\dagger_{\boldsymbol{r},B_1} c_{\boldsymbol{r},B_1} - c^\dagger_{\boldsymbol{r},A_3} c_{\boldsymbol{r},A_3} - c^\dagger_{\boldsymbol{r},B_3} c_{\boldsymbol{r},B_3} \right), \tag{10}$$

with $\Delta = 30\,\text{meV}$. We choose $n_s \times n_s = 18 \times 18$ as supercell size, with $N_{\boldsymbol{k}} = 24^2$ momentum points in the mini-BZ. The Fermi smoothening parameters are the same as in Section IV, as well as the energy/momentum space weighting parameters of the projected Wannier function guesses. Figure 4 (a) displays the absolute value of the two Wannier functions (for one valley $\nu = +$) individually on each of the six sites in the microscopic unit cell. The evolution of the envelope phase is shown in Fig. 4 (b). Finally, Fig. 5 demonstrates that the Wannier functions accurately reproduce the dispersion of ABC trilayer graphene. We note that this plot shows *both* valleys of the microscopic model (gray), but only *one* valley of the Wannier model (orange).

## VI. DUAL-GATED OHNO-COULOMB INTERACTION

With Wannier functions defined on the microscopic $p_z$ Wannier basis at hand, we may project the electronic Coulomb repulsion to the mesoscopic Wannier basis $\chi_{\zeta,\nu}$. First, we must define an appropriate interaction profile $V(r)$ in real space. The long-range tail is screened exponentially in dual-gate setups of recent experimental device architectures [1, 6]:

$$V_{\text{long}}(r) = 4V_0 \sum_{k=0}^{\infty} K_0 \left[ (2k+1)\pi \frac{r}{\xi} \right], \tag{11}$$

where $K_n(x)$ denotes a modified Bessel function of the second kind, $V_0$ sets the overall interaction strength, and $2\xi$ is the distance between the two gates [95]. The short-ranged part of the Coulomb interaction must also be screened when working with a lattice model. Thus we employ an Ohno potential [61]:

$$V_{\text{short}}(r) = \frac{U_0}{\sqrt{1 + r^2/a^2}}, \tag{12}$$

where we use $U_0 = 8.3\,\text{eV}$. Since the Ohno distance is on the order of $a \sim 1\,\text{Å}$, and gate distances are on the order of $\xi \sim 10\,\text{nm}$, we can safely assume to be in the limit where $a/\xi \to 0$.

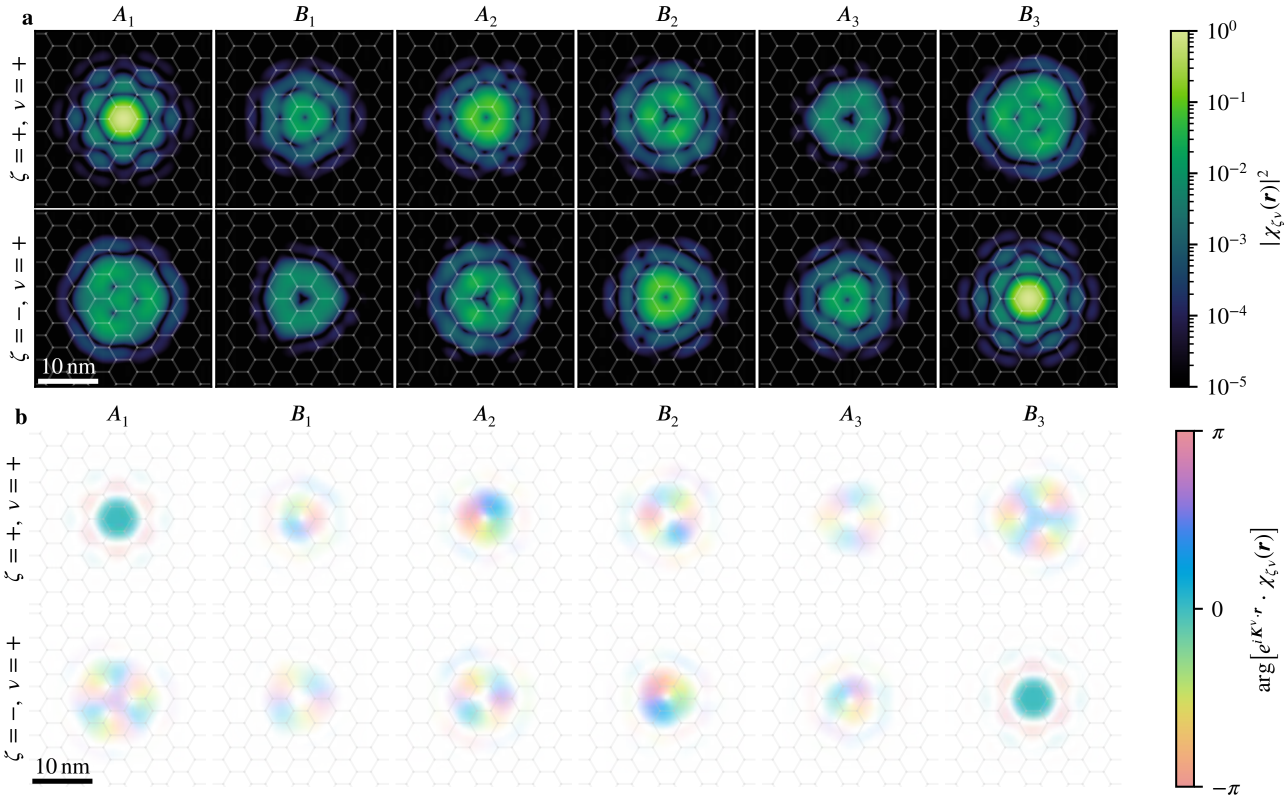


FIG. 4. Supercell Wannier functions of rhombohedral (ABC) trilayer graphene under the influence of an electric displacement field $\Delta = 30\,\mathrm{meV}$. (a): Absolute value of the two Wannier functions in real space for valley $\nu = +$ on the six sublattices. (b) Complex phase evolution of the envelope function, i.e., without the microscopic phase stemming from the valley.

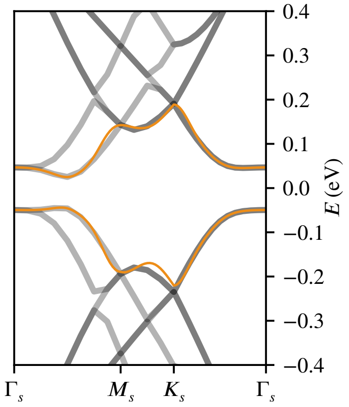


FIG. 5. Wannier interpolation (orange) of the supercell band structure (gray) of ABC trilayer graphene with $\Delta = 30\,\mathrm{meV}$ as perpendicular electric field.

Using the asymptotic properties of Eqs. (11) and (12),

$$V_{\mathrm{long}}(r) \cdot \left( \frac{V_0\, \xi}{r} \right)^{-1} = 1 + \mathcal{O}\left( \frac{r}{\xi} \right) , \tag{13}$$

$$V_{\mathrm{short}}(r) = \frac{U_0\, a}{r} + \mathcal{O}\left( \frac{a^2}{r^2} \right) , \tag{14}$$

we can replace $r$ in Eq. (11) by its short-ranged screened expression motivated from Eq. (12), i.e.,

$$r_{\text{short}} = \sqrt{a^2 + r^2}\,. \tag{15}$$

Plugging this together, we have

$$V(r) = 4V_0 \sum_{k=0}^{\infty} K_0 \left[ (2k+1)\pi \frac{\sqrt{r^2 + a^2}}{\xi} \right] , \tag{16}$$

which has the same long-range asymptotics as Eq. (11), and the same short-range behavior as Eq. (12), because the *long-range* behavior of Eq. (14) is just that of $1/r$, as well as the *short-range* behavior of Eq. (13).

In its final form, the Coulomb interaction Eq. (16) has no free parameters. The value of $\xi$ is set by the (experimental) gate distance. Thereafter, we observe that the Hubbard-$U$ must be obtained at $r = 0$. Together with Eq. (13), this yields

$$U = V_0 \frac{\xi}{a}\,. \tag{17}$$

The energy scale of the long-range tail, however, is fixed by the dielectric constant $\epsilon$. Since $\xi \gg a$, there is a regime where $\xi \gg r \gg a$. In this regime, the interaction behaves in its regular Coulomb way. Thus, we can again use the asymptotic expansion Eq. (13) and compare it to the Coulomb interaction in a dielectric background (hBN, $\epsilon \approx 4$):

$$V_0 \frac{\xi}{r} = \frac{\alpha}{\epsilon r}\,. \tag{18}$$

Equation (18) directly fixes $V_0$, and our sole choice to correctly reproduce the on-site Hubbard interaction $U$ of graphitic systems is to modify the Ohno parameter $a$ in a way that Eq. (17) is fulfilled. This yields

$$V_0 = \frac{\alpha}{\epsilon\xi}\,, \qquad a = \frac{\alpha}{\epsilon U}\,. \tag{19}$$

Our approach of orbitally resolved supercell Wannier functions allows to capture more complicated interaction profiles, and there is no conceptual problem in using, e.g., a cRPA [88] (or cFRG [89]) interaction profile as an input for the downfolding procedure.

## VII. VALLEY AS QUANTUM NUMBER

In any microscopic (graphitic) lattice model, valley order must be encoded through an order parameter that lives on *bonds* rather than *sites*. This is due to the fact that the valley operator $\mathcal{V}$ [77] intrinsically asks for hopping matrix elements rather than on-site components, i.e.,

$$\mathcal{V} = \frac{i}{3\sqrt{3}} \sum_{\langle\langle i,j \rangle\rangle} \eta_{ij} \sigma_z^{ij} c_i^\dagger c_j\,, \tag{20}$$

where $\langle\langle i,j \rangle\rangle$ runs over all next-nearest (in-plane) neighbors, $\eta_{ij}$ is $\pm 1$ for (counter) clockwise direction, and $\sigma_z$ acts in the space of sublattice (i.e. $A$, $B$). In order to transform Eq. (20) to momentum space, we have to write it in terms of lattice vectors $\boldsymbol{r}$, sublattice indices $i$, and bonds $\boldsymbol{b}_{\boldsymbol{r},i}^{\boldsymbol{r}',j}$. We show that the valley operator does *not* modulate the density, i.e., has no dependence on primary bilinear transfer momentum $\boldsymbol{q}$, but on the secondary momentum $\boldsymbol{k}$:

$$\mathcal{V} = \sum_{o \in \{A_1,\dots,B_N\}} \sigma_z^{oo} \frac{i}{3\sqrt{3}} \sum_{\boldsymbol{r}} \sum_{\boldsymbol{b}_{\boldsymbol{r},o}^{\boldsymbol{r}',o}} \eta_{\boldsymbol{b}} c_{\boldsymbol{r},o}^\dagger c_{\boldsymbol{r}+\boldsymbol{b},o} = \sum_{o \in \{A_1,\dots,B_N\}} \sigma_z^{oo} \frac{i}{3\sqrt{3}} \mathsf{V}_o \tag{21}$$

$$\begin{aligned} \mathsf{V}_o &= \sum_{\boldsymbol{r},\boldsymbol{b}_{\boldsymbol{r},o}^{\boldsymbol{r}',o}} \eta_{\boldsymbol{b}} \sum_{\boldsymbol{k}} e^{-i\boldsymbol{k}\boldsymbol{r}} c_{\boldsymbol{k},o}^\dagger \sum_{\boldsymbol{k}'} e^{i\boldsymbol{k}'(\boldsymbol{r}+\boldsymbol{b}_{\boldsymbol{r}}^{\boldsymbol{r}'})} c_{\boldsymbol{k}',o} = \sum_{\boldsymbol{k},\boldsymbol{k}',\boldsymbol{r},\boldsymbol{b}_{\boldsymbol{r},o}^{\boldsymbol{r}',o}} e^{i\boldsymbol{k}'\boldsymbol{r}+i\boldsymbol{k}'\boldsymbol{b}_{\boldsymbol{r}}^{\boldsymbol{r}'}-i\boldsymbol{k}\boldsymbol{r}} \eta_{\boldsymbol{b}} c_{\boldsymbol{k},o}^\dagger c_{\boldsymbol{k}',o} \\ &= \sum_{\boldsymbol{k},\boldsymbol{k}',\boldsymbol{r},\boldsymbol{b}_o} e^{i\boldsymbol{k}'\boldsymbol{r}+i\boldsymbol{k}'\boldsymbol{b}_o-i\boldsymbol{k}\boldsymbol{r}} \eta_{\boldsymbol{b}} c_{\boldsymbol{k},o}^\dagger c_{\boldsymbol{k}',o} = \sum_{\boldsymbol{k},\boldsymbol{b}_o} e^{i\boldsymbol{k}\boldsymbol{b}} \eta_{\boldsymbol{b}} c_{\boldsymbol{k},o}^\dagger c_{\boldsymbol{k},o} = \sum_{\boldsymbol{k}} \left( \sum_{\boldsymbol{b}_o} e^{i\boldsymbol{k}\boldsymbol{b}} \eta_{\boldsymbol{b}} \right) c_{\boldsymbol{k},o}^\dagger c_{\boldsymbol{k},o} = \sum_{\boldsymbol{k}} \eta_{\boldsymbol{k},o} c_{\boldsymbol{k},o}^\dagger c_{\boldsymbol{k},o}\,, \end{aligned} \tag{22}$$

where we used the fact that the bonds $\boldsymbol{b}_{\boldsymbol{r},i}^{\boldsymbol{r}',j}$ only depend on the sublattice index $o$. Equation (22) suggestively expresses the valley operator in the language of a nematic bilinear (also known in the context of a Pomeranchuck instability), making it clear that it,

in terms of a general Fermion bilinear $\langle c^\dagger_{\boldsymbol{q}+\boldsymbol{k}} c_{\boldsymbol{k}} \rangle$, represents a term that resides at $\boldsymbol{q} \equiv 0$. It can thus *never* be formulated through an on-site bilinear, no matter what basis transformation is chosen.

However, we can approximate the valley operator with $\mathcal{V}^{\boldsymbol{Q}}$:

$$\mathcal{V}^{\boldsymbol{Q}} = \sum_{o \in \{A_1,\ldots,B_N\}} \sigma_z^{oo} \frac{i}{3\sqrt{3}} \mathsf{V}_o^{\boldsymbol{Q}}, \qquad \mathsf{V}_o^{\boldsymbol{Q}} = \sum_{\boldsymbol{k}} \eta_{\boldsymbol{k},o} c^\dagger_{\boldsymbol{k}+\boldsymbol{Q},o} c_{\boldsymbol{k},o}, \tag{23}$$

where $|\boldsymbol{Q}| \ll |\boldsymbol{g}_i|$, with $\boldsymbol{g}_i$ the reciprocal lattice vectors. Equation (23) now corresponds to a Fermion bilinear that, besides its bond content $\eta_{\boldsymbol{k},o}$, has a modulated "density" component at momentum scale $\boldsymbol{Q}$. In the SWF language, we choose $\boldsymbol{Q} \in \{\boldsymbol{G}_1, \boldsymbol{G}_2, \boldsymbol{G}_3\}$ as the mesoscopic reciprocal lattice vectors that satisfy $|\boldsymbol{G}_i| \ll |\boldsymbol{g}_i|$, since the extent of the supercell is $n_s \gg 1$. Because the *approximate* valley operator $\mathcal{V}^{\boldsymbol{Q}}$ drops to zero at the Brillouin zone edges, one can choose a basis *within one supercell* where it is diagonal. This is automatically encoded in our Wannier trial states, because we take Bloch states from the original $\boldsymbol{K}^\nu$ points. Truncating the Wannier basis after a fixed number of trial states renders valley a quantum number in the Wannier basis. $U(1)$ valley symmetry of the projected model can therefore be understood to be *approximate* in the following sense: The valley operator is shifted from zero transfer momentum to $0 < |\boldsymbol{Q}| \ll |\boldsymbol{g}_i|$. Hence $U(1)$ becomes exact only in the infinite supercell limit (the continuum limit).


[44] J. Jung and A. H. MacDonald, Accurate tight-binding models for the $\pi$ bands of bilayer graphene, Physical Review B **89**, 035405 (2014).
[96] A. A. Mostofi, J. R. Yates, Y.-S. Lee, I. Souza, D. Vanderbilt, and N. Marzari, wannier90: A tool for obtaining maximally-localised wannier functions, Computer physics communications **178**, 685 (2008).
[93] K. Koepernik, O. Janson, Y. Sun, and J. Van Den Brink, Symmetry-conserving maximally projected wannier functions, Physical Review B **107**, 235135 (2023).
[92] M. Kang, S. Fang, L. Ye, H. C. Po, J. Denlinger, C. Jozwiak, A. Bostwick, E. Rotenberg, E. Kaxiras, J. G. Checkelsky, and R. Comin, Topological flat bands in frustrated kagome lattice CoSn, Nature Communications **11**, 4004 (2020).
[78] N. Marzari and D. Vanderbilt, Maximally localized generalized wannier functions for composite energy bands, Physical review B **56**, 12847 (1997).
[94] I. Souza, N. Marzari, and D. Vanderbilt, Maximally localized wannier functions for entangled energy bands, Phys. Rev. B **65**, 035109 (2001).
[68] S. Carr, S. Fang, H. C. Po, A. Vishwanath, and E. Kaxiras, Derivation of wannier orbitals and minimal-basis tight-binding hamiltonians for twisted bilayer graphene: First-principles approach, Phys. Rev. Res. **1**, 033072 (2019).
[97] F. Zhang, B. Sahu, H. Min, and A. H. MacDonald, Band structure of *abc*-stacked graphene trilayers, Phys. Rev. B **82**, 035409 (2010).
[6] A. M. Seiler, M. Statz, I. Weimer, N. Jacobsen, K. Watanabe, T. Taniguchi, Z. Dong, L. S. Levitov, and R. T. Weitz, Interaction-driven (quasi-) insulating ground states of gapped electron-doped bilayer graphene (2023), arXiv:2308.00827 [cond-mat.str-el].
[1] A. M. Seiler, F. R. Geisenhof, F. Winterer, K. Watanabe, T. Taniguchi, T. Xu, F. Zhang, and R. T. Weitz, Quantum cascade of correlated phases in trigonally warped bilayer graphene, Nature **608**, 298 (2022).
[95] R. E. Throckmorton and O. Vafek, Fermions on bilayer graphene: Symmetry breaking for b= 0 and $\nu$= 0, Physical Review B **86**, 115447 (2012).
[61] T. O. Wehling, E. Şaşıoğlu, C. Friedrich, A. I. Lichtenstein, M. I. Katsnelson, and S. Blügel, Strength of effective coulomb interactions in graphene and graphite, Phys. Rev. Lett. **106**, 236805 (2011).
[88] F. Aryasetiawan, M. Imada, A. Georges, G. Kotliar, S. Biermann, and A. Lichtenstein, Frequency-dependent local interactions and low-energy effective models from electronic structure calculations, Physical Review B **70**, 195104 (2004).
[89] M. Kinza and C. Honerkamp, Low-energy effective interactions beyond the constrained random-phase approximation by the functional renormalization group, Phys. Rev. B **92**, 045113 (2015).
[77] A. Ramires and J. L. Lado, Electrically tunable gauge fields in tiny-angle twisted bilayer graphene, Physical review letters **121**, 146801 (2018).
